# Supplementary material for: A coherence sweet spot with enhanced dipolar coupling
Source: arXiv:2405.10796 ancillary file (2024-05-30)
Supplement: Supplementary file 1 [file SM.pdf]

# Supplementary Material – A coherence sweet spot with enhanced dipolar coupling

J. H. Ungerer,[1,2,3,*] A. Pally,[2,†] S. Bosco,[4] A. Kononov,[2] D. Sarmah,[2] S. Lehmann,[5]
C. Thelander,[5] V.F. Maisi,[5] P. Scarlino,[6] D. Loss,[2] A. Baumgartner,[1,2] and C. Schönenberger[1,2,‡]

[1]*Swiss Nanoscience Institute, University of Basel, Klingelbergstrasse 82 CH-4056, Switzerland*
[2]*Department of Physics, University of Basel, Klingelbergstrasse 82 CH-4056, Switzerland*
[3]*Department of Physics, Harvard University, Cambridge, MA 02138, USA*
[4]*QuTech and Kavli Institute of Nanoscience, Delft University of Technology, Lorentzweg 1, 2628 CJ Delft, Netherlands*
[5]*Solid State Physics and NanoLund, Lund University, Box 118, S-22100 Lund, Sweden*
[6]*Institute of Physics and Center for Quantum Science and Engineering,
Ecole Polytechnique Fédérale de Lausanne, CH-1015 Lausanne, Switzerland*

In this supplementary, we discuss in detail the relevant theoretical considerations about the possible sources of decoherence that might give rise to the experimentally observed compromise-free sweet spot described in the main text.

## I. GENERAL FRAMEWORK FOR DECOHERENCE

In this Supplementary Material (SM), we investigate several possible origins of noise in order to pinpoint to the dominant noise source explaining the dependence of the experimentally measured decoherence. The investigate the deocherence of the ST transition, which consists in dephasing and relaxation,

$$\gamma = \frac{\gamma_1}{2} + \gamma_\varphi \ . \tag{1}$$

Generally for a two-level transition, we can model the noise by the effective Hamiltonian

$$H_N^D = \delta_z \frac{\tau_z}{2} + \delta_x \frac{\tau_x}{2} + \delta_y \frac{\tau_y}{2} \ , \tag{2}$$

where the index $D$ indicates that we are working in the diagonal basis of the two-level system, gapped by the energy $\Delta_{\mathrm{so}}$. The first term in $H_N^D$ causes pure dephasing (with decoherence rate $\gamma_\varphi$), while the second and third are responsible for relaxation (with rate $\gamma_1$).

By following Bloch-Redfield theory [1, 2], we find

$$\gamma_1 = \frac{1}{2\hbar^2}\int_{-\infty}^{\infty} d\tau \cos\left(\frac{\Delta_{\mathrm{so}}\tau}{\hbar}\right)\Big(\langle\delta_x(0)\delta_x(\tau)\rangle + \langle\delta_y(0)\delta_y(\tau)\rangle\Big) \ , \tag{3}$$

$$\gamma_\varphi = \frac{1}{2\hbar^2}\int_{-\infty}^{\infty} d\tau \langle\delta_z(0)\delta_z(\tau)\rangle \ . \tag{4}$$

Here, $\langle O(0)O(\tau)\rangle$ is the correlator of the operator $O$, typically evaluated for baths at thermal equilibrium. One can simplify these equations by introducing the spectral function of the noise

$$S_{ij}(\hbar\omega) = \int_{-\infty}^{\infty} d\tau e^{-i\omega\tau}\langle\delta_i(0)\delta_j(\tau)\rangle \ , \quad \langle\delta_i(0)\delta_j(\tau)\rangle = \frac{1}{2\pi}\int_{-\infty}^{\infty} d\omega e^{i\omega\tau} S_{ij}(\hbar\omega) \ , \tag{5}$$

resulting in

$$\gamma_1 = \frac{S_{xx}(-\Delta_{\mathrm{so}}) + S_{yy}(-\Delta_{\mathrm{so}}) + S_{xx}(\Delta_{\mathrm{so}}) + S_{yy}(\Delta_{\mathrm{so}})}{4\hbar^2} \tag{6}$$

$$\gamma_\varphi = \frac{S_{zz}(0)}{2\hbar^2} \ . \tag{7}$$

---

* Equal contributions.; jungerer@g.harvard.edu
† Equal contributions.
‡ nanoelectronics.unibas.ch

Note that one can estimate the effect of pure dephasing better by employing the filter function formalism, following Ref. [3]. For Gaussian noise and free induction decay, one finds that the decay of coherence is not generally exponential $e^{-t\gamma_\varphi}$, but follows the law

$$\exp\left[-\frac{1}{\pi\hbar^2}\int_{-\infty}^{\infty} d\omega S_{zz}(\hbar\omega)\frac{\sin^2(\omega t/2)}{\omega^2}\right] \ , \tag{8}$$

and agrees exactly with the result above (and with the exponential decay) for white noise $S_{zz}(\hbar\omega) \to S_{zz}(0)$.

We now adapt this theory to describe some possible mechanisms that produce noise in the system.

## II. TUNNELING AND DETUNING NOISE

Here, we explicitly calculate the decoherence for several noise sources, investigating whether the trend in $\gamma$ matches with the experimentally measured values. While doing so, we amplify the noise by a factor that might be reasonable depending on experimental circumstances. This allows us to exclude the particular noise source as dominant, if the trend does not match.

A possible decoherence mechanism is the coupling of charge traps and phonons to the tunneling and detuning of the DQD. The noise in this section is computed as follows: We first find the eigenstates of the DQD Hamitlonian in Eq. 13 of the main text. These eigenstates depend on B field amplitude and direction, as well as on detuning. Then we project the vairiaion of tunnelling and detuning (put in the equations 15 and 16 from Cleaner notes, and add the prefactor delta t(t) and delta epsilon (t) )) onto these eigenstates. Restricting ourselves to the subspace spanned by the ground and first excited state, we find the Hamiltonain in Eq. (2) and the dependence of the coupling to the noise sources $\delta_t$ and $\delta_\epsilon$ on detuning and B field. We then find the values at the anticrossing by evaluating at detuning values such that $\partial_\varepsilon(E_1 - E_0) = 0$. We neglect here the possible coupling of noise directly to the spin degree of freedom that might occur via an electric field tunable g-tensor and spin-orbit interaciton.

### A. 1/f charge noise

We consider the effect of an ensemble of random charge fluctuators coupling to the DQD. These impurities cause flucutations of the electrostatic potential $V$ that then couple to both $t_c$ and $\varepsilon$, and typically results in the noise spectrum

$$S_{tt}(\omega) = \int \mathrm{d}\tau e^{-i\omega\tau}\langle\delta_t(0)\delta_t(\tau)\rangle \tag{9}$$

$$= \left(\frac{\partial t}{\partial V}\right)^2 \bar{V}^2 \frac{\omega_0^{\alpha-1}}{|\omega|^\alpha} \ , \tag{10}$$

$$S_{\varepsilon\varepsilon}(\omega) = \int \mathrm{d}\tau e^{-i\omega\tau}\langle\delta_\varepsilon(0)\delta_\varepsilon(\tau)\rangle \tag{11}$$

$$= \left(\frac{\partial \varepsilon}{\partial V}\right)^2 \bar{V}^2 \frac{\omega_0^{\alpha-1}}{|\omega|^\alpha} \ , \tag{12}$$

with $\alpha \in (0, 2]$, $\omega_0 = 2\pi$ Hz being a reference frequency, and $\bar{V} \sim \mu$eV characterizing the amplitude of the noise.

Using these noise spectra, we numerically calculate the relaxation rates and dephasing rates due to noise coupling via the detuning and tunneling and plot the results in Figure 1. Tthe operators describing small variations of tunelling $t_c$ and detuning $\epsilon$ are given by

$$h_{\delta t} = \begin{pmatrix} \sin(2\theta) & -\cos(2\theta) & 0 & 0 & 0 \\ -\cos(2\theta) & -\sin(2\theta) & 0 & 0 & 0 \\ 0 & 0 & 0 & 0 & 0 \\ 0 & 0 & 0 & 0 & 0 \\ 0 & 0 & 0 & 0 & 0 \end{pmatrix} \ , \tag{13}$$

$$h_{\varepsilon} = \begin{pmatrix} -\sin^2(\theta) & \sin(2\theta)/2 & 0 & 0 & 0 \\ \sin(2\theta)/2 & -\cos^2(\theta) & 0 & 0 & 0 \\ 0 & 0 & 0 & 0 & 0 \\ 0 & 0 & 0 & 0 & 0 \\ 0 & 0 & 0 & 0 & 0 \end{pmatrix} \ . \tag{14}$$

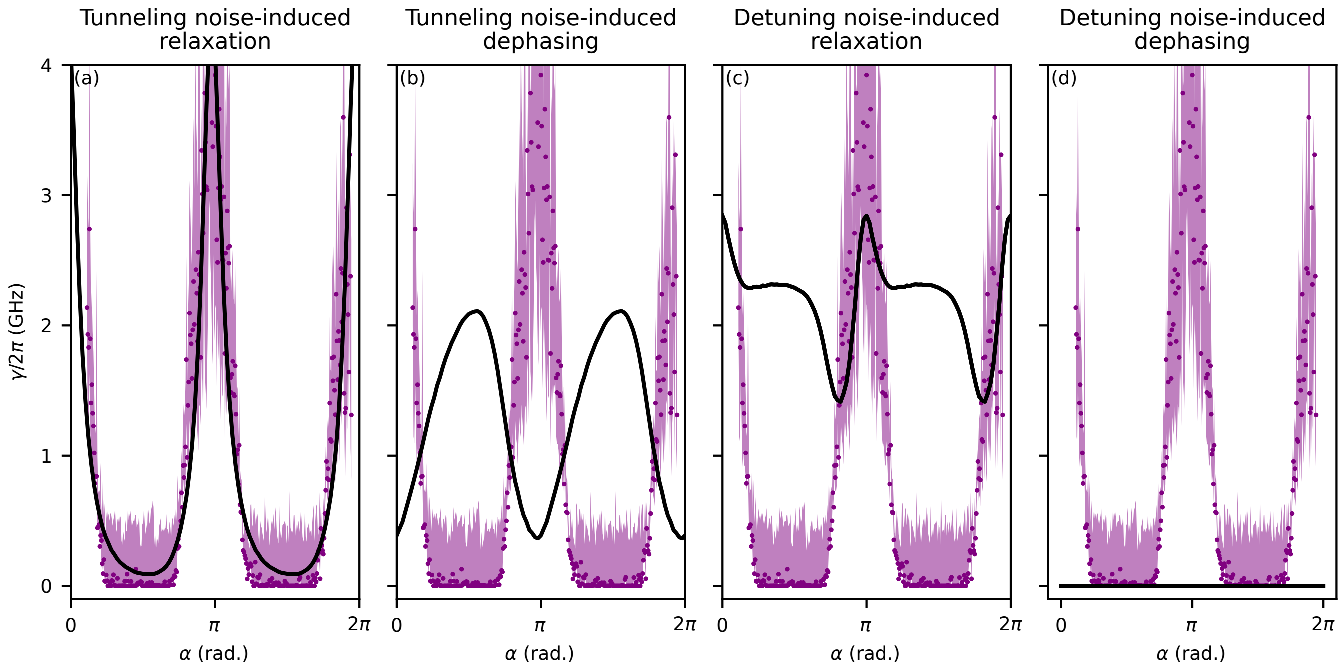


FIG. 1. **Pink ($1/f$) noise.** All subfigures show the experimental data for the total dephasing rates (purple). The overlaid curves are **(a)** Black curve represents the relaxation rate due to pink noise coupling to the tunnel rate, $\gamma_1^{t,1/f} = \frac{|h_{\delta t01}|^2 S_{tt}(\Delta_{\rm so})}{4\hbar^2}$. **(b)** Black curve represents the dephasing due to pink noise coupling to the tunnel rate $t_c$, $\gamma_\varphi^{t,1/f} = \sqrt{2 \cdot 3.5}\,(\langle 0| h_{\delta t} |0\rangle - \langle 1| h_{\delta t} |1\rangle)$. **(c)** Black curve represents the relaxation due to pink noise coupling to the detuning $\varepsilon$, $\gamma_1^\varepsilon = \frac{|h_{\delta\epsilon 01}|^2 S_{\epsilon\epsilon}(\Delta_{\rm so})}{4\hbar^2}$. **(d)** Black curve represents represents the dephasing due to pink noise coupling to the detuning $\varepsilon$, $\gamma_\varphi^\varepsilon = 0$. This term vanishes because it was evaluated at the avoided crossing, where $\partial(E_1 - E_0)/\partial\varepsilon = 0$.

The definitions of these operators leads to the matrix elements

$$h_{\delta t01} = \langle 0| h_{\delta t} |1\rangle \ \ , h_{\delta tz} = \frac{\langle 0| h_{\delta t} |0\rangle - \langle 1| h_{\delta t} |1\rangle}{2} \ , h_{\delta\epsilon 01} = \langle 0| h_{\delta\epsilon} |1\rangle \ \ , h_{\delta\epsilon z} = \frac{\langle 0| h_{\delta\epsilon} |0\rangle - \langle 1| h_{\delta\epsilon} |1\rangle}{2} \ , \tag{15}$$

where $|0\rangle$ and $|1\rangle$ are the qubit states. We note that, by construction, noise coupling via the detuning $\varepsilon$ does not cause dephasing because the noise is evaluated at the position of the avoided crossing where $\partial_\varepsilon(E_1 - E_0) = 0$. The relaxation rate due to pink noise coupling to the tunnel rate is then given by,

$$\gamma_1^{t,1/f} = \frac{|h_{\delta t01}|^2 S_{tt}(\Delta_{\rm so})}{4\hbar^2} \tag{16}$$

and the relaxation due to pink noise coupling via the detuning reads

$$\gamma_1^\epsilon = \frac{|h_{\delta\epsilon 01}|^2 S_{\epsilon\epsilon}(\Delta_{\rm so})}{4\hbar^2} \ . \tag{17}$$

We then estimate the decay as Gaussian (see Eq. (8)), rather than exponential. Neglecting log corrections leads to the dephasing due to pink noise coupling to the tunnel rate

$$\gamma_\varphi^{t,1/f} \approx \frac{1}{\hbar}|h_{\delta tz}|\bar{V}\frac{\mathrm{d}t}{\mathrm{d}V} \ , \tag{18}$$

and the dephasing due to pink noise coupling to the detuning

$$\gamma_\varphi^{\varepsilon,1/f} \approx \frac{1}{\hbar}|h_{\delta\epsilon z}|\bar{V}\frac{d\varepsilon}{\mathrm{d}V} \ . \tag{19}$$

These quantities from Eqs. (16), (17), (18) and (19) are plotted as curves overlaid over the decoherence rate extracted from the measurements in Fig. 1. From the curves, it becomes obvious that when considering pink noise, only

relaxation due to coupling via the tunnel rate $t_c$ results in the trend that is observed in the experimental data. However, if this was the main source of noise, the total decoherence rate would be the sum of the the dephasing and the relaxation terms (Fig. 1(a) and (b), thus providing a globally different trend than what observed in the experiment.

### B. Phonons

We consider two types of phonon interactions, whose energy is determined by their strain tensor $\varepsilon$. Deformational phonon interactions create a potential via longitudinal terms in the strain tensor

$$H_D = \varepsilon_D \mathrm{Tr}(\varepsilon) \ , \tag{20}$$

while piezoelectric phonon interactions introduce in the system an electric field $\mathbf{E}_s$ via the shear strain tensor elements, which results in

$$H_P = -e \int d\mathbf{r}' \frac{(\nabla \cdot \mathbf{E}_s)(\mathbf{r}')}{|\mathbf{r}-\mathbf{r}'|} \ , \tag{21}$$

$$\mathbf{E}_s = E_P \begin{pmatrix} \varepsilon_{yz} \\ \varepsilon_{xz} \\ \varepsilon_{xy} \end{pmatrix} \ . \tag{22}$$

We ignore here the vector potential contributions of $\mathbf{E}_s$. The energy $\varepsilon_D \sim 14$ eV, and the piezoelectric electric field $E_P \sim 0.1$V/nm are material-dependent parameters.

The tunneling and detuning fluctuations caused by these phonons are then given by

$$\delta t_{D,P} = 2\langle\Psi_L|H_{D,P}|\Psi_R\rangle \ , \quad \delta\varepsilon_{D,P} = \langle\Psi_L|H_{D,P}|\Psi_L\rangle - \langle\Psi_R|H_{D,P}|\Psi_R\rangle \ , \tag{23}$$

where $|\Psi_{L,R}\rangle$ are the orthonormalized electronic wavefunctions of the left and right dots. We note that here $\delta t_{D,P}$ and $\delta\varepsilon_{D,P}$ are operators and thus the phonons spectral function is generally asymmetric in frequency, causing quantum noise (see e.g. Ref. [4]). Moreover, because the phonons spectral function vanishes at $\omega = 0$, we restrict ourselves to the analysis of the dominant contribution of phonons to decoherence that is relaxation.

We also focus on the tunneling and detuning flucutations caused by phonons confined in a 1 dimensional nanowire. We consider here a simplified model of the nanowire based on continuous elasticity theory in isotropic medium, which assumed the wire to be infinitely long (formally with a length $L \to \infty$) and cylindrical with radius $R$. There are four phonon modes: longitudinal, transversal, and two flexural modes. The longitudinal mode contributes via both piezoeletric and deformational interactions, while the others only via piezoelectric ones.

However, by following closely Ref. [5], we find that the shear strain components $\varepsilon_{ij}$ of the different modes oscillate around the nanowire and thus their contribution averages to zero if the electronic wavefunction is cylindrical. These interactions qualitatively capture the trends observed in experiment. We note that piezoelectric phonon coupling vanishes in our simplified model, but it can still be quantitatively relevant in experiments if one includes non-cylydnrical and finite length nanowires and anisotropic elastic media. We also neglect here the effect of the difference of materials in the wire, which could have an effect to modify the phonon-quibit itneractions. For this reason, we expect that the dominant contribution of the phonons is caused by longitudinal phonon modes coupled via deformational interactions.

Assuming the electronic wavefunctions to be Gaussians of width $l$, shifted by a distance $d$, orthonomalized as

$$\begin{pmatrix} \langle\mathbf{r}|\Psi_R\rangle \\ \langle\mathbf{r}|\Psi_L\rangle \end{pmatrix} = \frac{e^{-(x^2+y^2)/2R^2}}{\sqrt{\pi}R} \frac{1}{2\sqrt[4]{\pi l^2}} \begin{pmatrix} \frac{1}{\sqrt{1+s}} + \frac{1}{\sqrt{1-s}} & \frac{1}{\sqrt{1+s}} - \frac{1}{\sqrt{1-s}} \\ \frac{1}{\sqrt{1+s}} - \frac{1}{\sqrt{1-s}} & \frac{1}{\sqrt{1+s}} + \frac{1}{\sqrt{1-s}} \end{pmatrix} \begin{pmatrix} e^{-(z-d)^2/2l^2} \\ e^{-(z+d)^2/2l^2} \end{pmatrix} \ , \tag{24}$$

with $s = e^{-d^2/l^2}$, we obtain from Eq. (23) [and using Eqs. (78)-(80) and (98) in Ref. [5]]

$$\delta\varepsilon_D = \varepsilon_D(1-2\nu)\frac{1}{\sqrt{1-e^{-2d^2/l^2}}} \sum_q \sqrt{\frac{2\hbar}{\pi L R^4 \rho c_l |q|}} |q| R e^{-q^2 l^2/4} \sin(|q|d)[a_q^\dagger + a_q] \ , \tag{25}$$

$$\delta t_D = \varepsilon_D(1-2\nu)\mathrm{csch}\left(\frac{d^2}{l^2}\right) \sum_q \sqrt{\frac{2\hbar}{\pi L R^4 \rho c_l |q|}} |q| R e^{-q^2 l^2/4} \sin^2\left(\frac{|q|d}{2}\right) [a_q^\dagger + a_q] \ , \tag{26}$$

which results in the relaxation time

$$\gamma_1^{ph} = \gamma_1^{\epsilon} + \gamma_1^{t} \tag{27}$$

$$\gamma_1^{i} = \Gamma_{\rm ph}|h_{\delta i01}|^2 \coth\left(\frac{\Delta_{\rm so}}{2\hbar kT}\right) F_i\left(\frac{\Delta_{\rm so}}{\hbar c_l}\right) \ , \tag{28}$$

$$F_{\varepsilon}(q) = |q|Re^{-q^2l^2/2}\frac{1}{1-e^{-2d^2/l^2}}\sin^2(|q|d) \ , \tag{29}$$

$$F_t(q) = |q|Re^{-q^2l^2/2}{\rm csch}^2\left(\frac{d^2}{l^2}\right)\sin^4\left(\frac{|q|d}{2}\right) \ . \tag{30}$$

Here, $c_l \approx 3\times10^3$ m/s is the phase velocity of the longitudinal phonons with wavevector $q$, $\rho = 5.5$ g/cm$^3$ is the density, and $\nu = 0.3$ is the Poisson ratio. We assumed that the phonons are in a thermal state with temperature $T$. When evaluating the expectation values of the phonon operators, we used $\langle a_q^\dagger a_{q'}\rangle = \delta_{qq'}N(\omega_q)$, $\langle a_q a_{q'}^\dagger\rangle = \delta_{qq'}[1 + N(\omega_q)]$ [with $N(x) = 1/(e^{\hbar x/k_BT} - 1)$], and $a_q^\dagger(\tau) = a_q^\dagger e^{i\omega_q\tau}$, $a_q(\tau) = a_q e^{-i\omega_q\tau}$. We also made use of the equality $1+2N(x) = \coth(\hbar x/2k_BT)$, and we converted the sum over discrete momenta to the integral $\int dqL/(2\pi)$. The coupling to detuning and tunnelling are related to the decoherence of the qubit by the procedure discussed above, which involves the projection of $h_{\delta t}$ and $h_{\delta\epsilon}$ hamiltonian to the qubit subspace. We note that the phonon-mediated relaxation rate $\Gamma_{\rm ph}$ can be estimated as

$$\Gamma_D = \frac{\varepsilon_D^2(1-2\nu)^2}{2\pi\hbar R^3\rho c_l^2} \approx 200\,{\rm MHz}, \tag{31}$$

when $R \sim 50$ nm. This is consistent with previous estimations [6] and in reasonable agreements with charge-like experiments in a similar device.

The theoretical curves in Fig. 3(e) and Fig. 4(a) corespond to Eq. (28) with numerically calculated matrix elements $|h_{\delta\varepsilon01}(\alpha)|$, $|h_{\delta t_c01}|(\alpha)$. To plot the curve plotted in Fig. 4(b), we fix $|h_{\delta\varepsilon01}| = |h_{\delta t_c01}| = 0.7$ to derive an analytical equation $\gamma_1^{\rm ph}(\omega)$. While the trend captured by the phonon dispersion nicely reproduces the features observed in the experiment, we note that $\Gamma_{\rm ph} = 240\,{\rm GHz}$ , extracted from our measurement, and setting the largest decay rate, is significantly larger than $\Gamma_{\rm D}$. This discrepancy could be due to the physical structure of the nanowire, for example the tunnel barrier between the two dots could modify the phonon-qubit coupling Also, the non-perfectly one-dimensional nature of the wire could be relevant. Another possibility to explain the larger $\Gamma_D$ is that, we are close to a phonon-relaxation hotspot, that can arise at the frequencies where higher phonon modes become populated. We estimate that the higher modes become populated at frequencies $\sim c_l/2R \sim 30$ GHz [6], not too far from the values of $\Delta_{\rm so}$ in our experiment. Fig. 2 shows the relaxation caused by phonons. Fig. 2(a) is equivalent to Fig. 3(e) and Fig. 4(a) in the main text and shows the relaxation mediated by phonons coupling to the tunneling. Fig. 2(b) shows the phonon-induced relaxation due to coupling via the detuning. We speculate that the the fact that the barriers are built of wurtzite InAs, compared to the zincblende InAs quantum dots, results in large phonon-induced variations of the tunnel coupling.

## III. NUCLEAR SPIN NOISE

We consider magnetic noise, such as nuclear spin noise, as source of decoherence. To model this noise source, we introduce here the fluctuations $\delta\mathbf{B}_N^{L,R}$ of the magnetic field in the left and right dots, which result in

$$\delta\mathbf{b}^N = \frac{\mu_B}{2}\left[\delta\mathbf{B}_N^L\underline{g}_L\underline{R}(-\theta_{\rm so}/2) - \delta\mathbf{B}_N^R\underline{g}_R\underline{R}(\theta_{\rm so}/2)\right] \ , \tag{32}$$

$$\bar{\mathbf{b}}^N = \frac{\mu_B}{2}\left[\delta\mathbf{B}_N^L\underline{g}_L\underline{R}(-\theta_{\rm so}/2) + \delta\mathbf{B}_N^R\underline{g}_R\underline{R}(\theta_{\rm so}/2)\right] \ , \tag{33}$$

and produce the magnetic noise Hamiltonian

$$H_M = \begin{pmatrix} 0 & 0 & \frac{-(\delta b_x^N + i\delta b_y^N)\cos(\theta)}{\sqrt{2}} & \frac{(\delta b_x^N - i\delta b_y^N)\cos(\theta)}{\sqrt{2}} & \delta b_z^N\cos(\theta) \\ 0 & 0 & \frac{-(\delta b_x^N + i\delta b_y^N)\sin(\theta)}{\sqrt{2}} & \frac{(\delta b_x^N - i\delta b_y^N)\sin(\theta)}{\sqrt{2}} & \delta b_z^N\sin(\theta) \\ \frac{-(\delta b_x^N - i\delta b_y^N)\cos(\theta)}{\sqrt{2}} & \frac{-(\delta b_x^N - i\delta b_y^N)\sin(\theta)}{\sqrt{2}} & \bar{b}_z^N & 0 & \frac{\bar{b}_x^N - i\bar{b}_y^N}{\sqrt{2}} \\ \frac{(\delta b_x^N + i\delta b_y^N)\cos(\theta)}{\sqrt{2}} & \frac{(\delta b_x^N + i\delta b_y^N)\sin(\theta)}{\sqrt{2}} & 0 & -\bar{b}_z^N & \frac{\bar{b}_x^N + i\bar{b}_y^N}{\sqrt{2}} \\ \delta b_z^N\cos(\theta) & \delta b_z^N\sin(\theta) & \frac{\bar{b}_x^N + i\bar{b}_y^N}{\sqrt{2}} & \frac{\bar{b}_x^N - i\bar{b}_y^N}{\sqrt{2}} & 0 \end{pmatrix} . \tag{34}$$

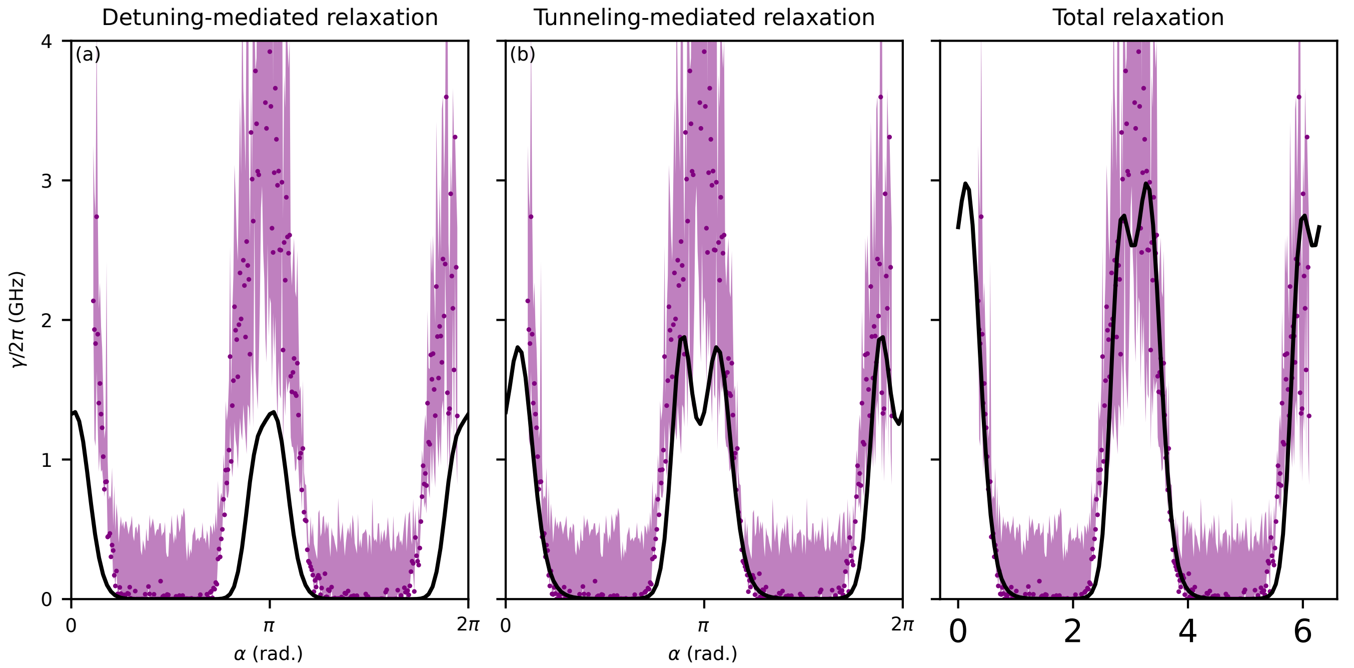


FIG. 2. **Phonon-mediated noise.** Both subfigures show the experimental data for the total dephasing rates (purple). **(a)** Black curve represents relaxation due to phonons-mediated tunnelling, $\gamma_1^{t_c}/2$ **(b)** Black curve represents relaxation due to phonons-mediated detuning, $\gamma_1^{\varepsilon}/2$. Both quantities are given by Eq. (28), where $i = t_c, \varepsilon$. **(c)** Total phonon-mediated relaxation $\gamma_1^{\rm ph}/2 = \gamma_1^{t_c}/2 + \gamma_1^{\varepsilon}/2$

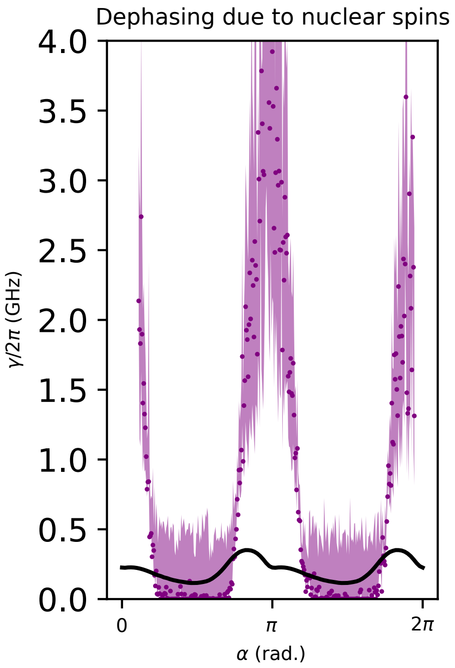


FIG. 3. **Hyperfine interaction-mediated noise.** Dephasing noise due to magnetic nosie from the nuclear spin bath. The solid curve is given by $\sqrt{\langle \delta_z^N \delta_z^N \rangle}/\sqrt{2}\hbar$. For plotting the black curve, we use a larger value of $1/\tau$ than expected to magnify the trend of the nuclear-spin induced noise.

Here the quantization axes are aligned to the total Zeeman energy, but we omit the index $'$ to simplify the notation.

To model the nuclear spins, we assume that the magnetic fields in the two dots differ by a random amount, thus leading to decoherence. The dynamics of the nuclear spins is typically slow and has low amplitude at large frequencies, and we restrict ourselves to the description of the dephasing rates and model the nuclear spin as sources of quasi-static noise, with spectral function $S_{\varphi\varphi} = \pi\delta(\omega)\hbar^2\Gamma_N^2$. This noise produces the typical Gaussian decay $e^{-\Gamma_N^2 t^2}$, rather than exponential.

To evaluate the rate $\Gamma_N = \sqrt{\langle \delta_z^N \delta_z^N \rangle}/\sqrt{2}\hbar$, we follow the same procedure used above and we project $H_M$ onto the lowest spin states in order to find the noise Hamiltonian $H_N^D$ in Eq. (2). We then assume uncorrelated and isotropic noise identical in amplitude in both dots, i.e. $\mu_B^2\langle(\delta\mathbf{B}_N^i)_n(\delta\mathbf{B}_N^j)_m\rangle = \delta_{ij}\delta_{mn}\hbar^2/\bar{\tau}^2$, such that

$$\mu_B^2\langle(\delta b_N)_n(\delta b_N)_m\rangle = \mu_B^2\langle(\bar{b}_N)_n(\bar{b}_N)_m\rangle = \frac{\hbar^2}{4\bar{\tau}^2}(\underline{B}_{nm}^L + \underline{B}_{nm}^R) \ , \tag{35}$$

$$\mu_B^2\langle(\delta b_N)_n(\bar{b}_N)_m\rangle = \frac{\hbar^2}{4\bar{\tau}^2}(\underline{B}_{nm}^L - \underline{B}_{nm}^R) \ , \tag{36}$$

$$\underline{B}^{L,R} = \underline{R}^T(\mp\theta_{\text{so}}/2)\underline{g}_{L,R}^T\underline{g}_{L,R}\underline{R}(\mp\theta_{\text{so}}/2) \ . \tag{37}$$

We overlay the results of the numerical calculation on the data in Figure 3 and note that it does not capture the order-of-magnitude dependence on the $B$-field alignment. Interestingly, we observe a similar anti-correlation with respect to the coupling to resonator, although with a much smaller amplitude of oscillation compared to the experimentally measured one. This gives us confidence that the compromise-free sweet spot makes the qubit more resilient against also against nuclear spin noise.

An alternative way to find an upper limit of the nuclear spin-induce decoherence is to consider the characteristic rate $\bar{\tau}$. We estimate the expected value as $\bar{\tau}^{-1} \approx \sqrt{\sum_k \nu_k I_k(I_k+1)A_k^2/\hbar^2 N}$, where $N \sim 10^8$ is the number of atoms in the dot and $\nu_k$ the percentage of spinful nuclei $k$ with spin $I_k$ and hyperfine coupling $A_k \sim 300$ $\mu$eV. We then find that $\Gamma_N \propto 1/\bar{\tau} \sim 0.1$ GHz which is much lower than the measured decoherence for fields perpendicular to the nanowire.

## IV. CONCLUSION

The calculations of the decoherence for various decoherence sources allow to exclude most of them as dominant in our experiments. By matching the trend expected by theoretical estimation with our measurement, we conclude that only magnetic noise stemming from nuclear spins and phonons are consistent with the experimental data.

[1] V. N. Golovach, A. Khaetskii, and D. Loss, Physical review letters **93**, 016601 (2004).
[2] V. Kornich, C. Kloeffel, and D. Loss, Quantum **2**, 70 (2018).
[3] Ł. Cywiński, R. M. Lutchyn, C. P. Nave, and S. D. Sarma, Physical Review B **77**, 174509 (2008).
[4] J. Zou, S. Bosco, and D. Loss, npj Quantum Information **10**, 46 (2024).
[5] C. Kloeffel, M. Trif, and D. Loss, Physical Review B **90**, 115419 (2014).
[6] M. Trif, V. N. Golovach, and D. Loss, Physical Review B **77**, 045434 (2008).
